# Supplementary material for: Secure Mobile Identities
Source: arXiv:1604.04667 source file (2016-04-16)
Supplement: Supplementary file 1 [file Appendix.tex]

\newpage
\appendix

\section{Why Not AppSec?}
\label{netsec}

As explained in \S \ref{threats}, there are a variety of issues that plague the communication network, affecting the applications that lie atop. Across the years, a variety of solutions have been proposed to detect and prevent adversarial action \cite{enck2011study,yoder1998architectural,huang2003web,stallings1995network,kaufman2002network,heberlein1990network}. While some of these solutions are at the application-level, others are at the network-level. The network is a very optimized resource that is commonly available, whilst applications are engineered as per demands; a practice that is ever maturing. Such applications are prone to a myriad of human-errors and loopholes present in the code \cite{durumeric2014matter,leyden2014patch,van2014learning,nohl2014badusb}. A survey by $7safe$ analyzing $62$ cybercrimes states that $86\%$ of the attacks stem from a weakness in the web interface. XSS attacks, Cookie Poisoning, and Hidden field manipulation are some examples of easy to execute threats to application level security resulting from the unauthorized usage of the applications. Given the large number of applications that exist today, we believe that enhanced security in the unifying layer would benefit developers, end users and service providers alike. 

\section{Using Untrusted Locations}
\label{usage}

If mobile device $U_1$ initiates a key exchange with device $U_2$ at a random time, then the location declared by $U_2$ is a (probabilistically) relevant untrusted location for $U_1$ but the inverse does not hold. To elaborate, $U_1$ queried the location of $U_2$ at a random time, and if $U_2$ is genuinely connected to the network, then the location reported by it does have benefit for $U_1$ as it is not modified by a party in the middle. On the other hand, if $U_1$ initiates key-exchange and self-declares its location, $U_2$ need not trust the declared location since it is unsure if $U_1$ initiated the key-exchange or if an fBTS did. This is inherently due to the asymmetry of the POWT Channel assumption, where the sender identity is not as trustworthy as the recipient. 

\section{Threshold Selection} 
\label{App:AppendixA}

Assume the probability of adversarial interferene at any location to be $p$. The successful completion of an epoch leads to a corresponding reputation score increase by an average value of $m$. As explained, the value of $m$ depends on whether the diverse locations in the epoch were trusted or untrusted and the corresponding weightage to them is accounted for in the reputation scoring functions. Successful completion of $L$ epochs (each requiring $k$ successful message exchanges) leads to a net increase in reputation of $L \times m$. Ideally, we would choose a reputation threshold $\Delta$ such that $(1-p)^{Lk} > p^{\Delta}$. Reducing further, we obtain $Lk \times l(p) \ < \Delta $ for a monotonically increasing function $l(p) = log(1-p)/log(p)$. In essence, for successful authentication, mobile nodes need to maintain a reputation $\Delta > Lk \times m$ where the average growth in reputation $m$ reflects the value of $p$.

\section{Implementation Details}
\label{micro}

We conducted simple micro benchmark tests on the message length, delivery delays and energy consumption across a real-world mobile networks in both UAE and the USA. The key observations are as follows:

\vspace{1mm}
{\em 1. Message Length:} We aim to reduce the length of messages using standard lossless compression techniques. The average length of a message required for the three-way handshake is 1640 characters before compression and 1364 after. This number can be further reduced by reducing the precision of information to be shared. As explained earlier, non-sensitive information such as unique user identifiers can be shared using alternate channels, decreasing the load shared through the SMS channel. 

\vspace{1mm}
{\em 2. Delivery Delay:} Delay in delivery is proportional to the length of the message. It was observed that the delay is 7.4 seconds using T-Mobile in the USA and 7.1 seconds using Etisalat in the UAE for a message of size 160 characters and scales linearly with the increase in message size. The deviation between the two countries is due to a combination of factors including the allocation of network infrastructure in the specific city of testing, fairness from service providers, coverage and network capacity.

\vspace{1mm}
{\em 3. Energy Consumption:} We used a Google Nexus 5 device (2300 mAh power supply) running Android v5.1.1 (Lollipop) to conduct spatio-temporal key-exchanges using just the SMS channel, with an aggressive periodicity of 5 minutes. This was done whilst default mobile applications were also running. We observed that the energy consumption was moderate; the SMI protocol execution resulted in roughly a 30\% decrease in battery (from full charge) after a 5.2 hour execution of the protocol which we believe is within acceptable energy boundaries as an {\em extreme} case (involving 310 key-exchanges). In practice, due to the use of multiple channels to achieve a much lower frequency of exchanges, the energy consumption will be much lower. We also believe the energy consumption will further decrease due to recent advancements in the design of new battery technologies \cite{yang2011improving}, and Android upgrades \cite{nexus,nexus2}.
