# Supplementary material for: Secure Mobile Identities
Source: arXiv:1604.04667 source file (2016-04-16)
Supplement: Supplementary file 2 [file 7-Additional.tex]

\section{Discussion}
\label{discussion}

We now discuss the rationale behind our design.
\vspace{-2mm}
\subsection{Trusted Location Distrbution}
\label{tld}

309 retailers have an estimated 7623 stores in New York City \cite{survey}. With a size of 304.6 sq. miles, the average store density is 25 stores/sq. mile. The zip code 10003 (Greenwich Village) of size 0.58 sq. miles has 164 retail stores, resulting in value of 282 stores/sq.mile in this area. This is 11 times the city-wide average and is attributed to the high population density of Manhattan and it being a popular tourist destination. The recent proliferation of NFC based payment has resulted in a large number of stores adapting contact-less payment solutions. Based on analysis, close to 80\% of the chosen stores in New York have use such solutions and are hence are location verified \cite{mastercard}. 
%That is to say, 8 in 10 stores one would visit is a trusted location.

\vspace{-2mm}
\subsection{Smartphone Proliferation}
\label{proliferation}

Based on a Pew survey, 64 \% of all US adults now have smartphones. However, among the population of mobile phone owners (91 \% of US adults), the smartphone penetration number is now 61 \%. Apple iPhone sales alone exceeded 40 million in the US for the 2014 financial year. 19\% of Americans rely to some degree on a smartphone for accessing online services and information-either because they lack broadband at home, or because they have few options for online access other than their cell phone.
\vspace{-2mm}
\subsection{Economic Implications}
\label{economics}

Another Pew survey suggests cell owners between the ages of 18 and 24 exchange an average of 109.5 messages on a normal day which works out to more than 3,200 texts per month. The typical or median cell owner in this age group sends or receives 50 messages per day (or 1500 messages per month). However, over 100 service providers in the United States provide unlimited messaging as part of their monthly plans \cite{whistleout}. This greatly alleviates the cost associated with the large number of messages exchanged between users of SMI.
\vspace{-2mm}
\subsection{Human Mobility}
\label{mobility}

The average moderately active person take aound 7500 steps per day. Doing the math; the average person with the average stride walks 3.76 miles a day. To support this claim, New York was voted the most active state in the US, according to a recent study from Fitbit, where a resident takes an average of 10000 steps per day.
%\subsection{QoS In Cellular Networks}
%
%A variety of factors affect the time taken to successfully deliver a message. Delays are caused due to:
%\vspace{-2mm}
%\begin{itemize}[leftmargin=-.01in]
%\itemsep-0.23em
%\item Low quality cellular devices.
%\item Delay in allocation of adequate network infrastructure.
%\item Lack of fairness from service providers.
%\item Limited coverage and network capacity.
%\item Poor government monitoring on standards.
%\item Environmental materials and current location i.e. distance from the cellular towers.
%\end{itemize}
%\vspace{-2mm} 
%Any combination of the afforementioned reasons could result in a deviation from optimal delivery time of the messages required for the SMI protocol. For example, the difference in message delivery time between AT$\&$T in New York City and Etisalat at Abu Dhabi may arise due differences in city demographics, geographics and infrastructure. This could cause advancements or delays towards the time required to build sufficient reputation. 
